# Supplementary material for: Cross Pairwise Ranking for Unbiased Item Recommendation
Source: arXiv:2204.12176 source file (2022-04-26)
Supplement: Supplementary file 1 [file 8_appendix.tex]

\appendix

\section{Appendix}

Optionally include extra information (complete proofs, additional experiments and plots) in the appendix.
This section will often be part of the supplemental material.
